# Supplementary material for: Education for expanding the quantum workforce: Student perceptions of the quantum industry in an upper-division physics capstone course
Source: arXiv:2407.07902 source file (2024-06-26)
Supplement: Supplementary file 2 [file Supp.pdf]

# Supplemental Materials for “Education for expanding the quantum workforce: Student perceptions of the quantum industry in an upper-division physics capstone course”

## I. FIRST INTERVIEW PROTOCOL

The following are the relevant parts of the interview protocol that was used for semi-structured interviews at the beginning of the first semester of Q-Forge.

### Background

- As we get started, I was curious what made you decide to take this Quantum Forge course? What are you expecting to get out of it?
- What are your plans for when you graduate from CU? What type of job are you looking for? What types of jobs do you know you are not interested in? How do you think Q-Forge will play into your plans of [their post CU plans mentioned above]?
- What quantum-focused courses have you taken?
- Have you taken any engineering lab courses?
- Have you had any prior research experiences? If so, can you tell me more about those experiences?
- Have you had any industry experiences? If so, can you tell me more about those experiences?
- What is your major and minors, if you have them?

### Quantum Industry Specific Questions

- Tell me a little bit about what you understand the quantum industry to be. Where did you learn what you currently know about the quantum industry? Do you know of any companies in the quantum industry? If yes, which ones do you know about? Do you know what types of jobs exist in the quantum industry? If yes, describe some of those jobs. Do you know what skills are required to work in the quantum industry? If yes, what are they?
- Are you interested in pursuing a job in the quantum industry? Why or why not? What influenced this interest? What kind of job would you like to pursue in the quantum industry? What parts of a job in quantum industry do you think you'd find interesting? What parts would you expect not to like? How does this compare with your interest in other options (e.g., other areas of industry, academia, etc.)?
- Do you think you will be able to get a job in the quantum industry? Explain. What do you see as the biggest challenge to getting a job in the quantum industry?
- Do you think you have the skills you need to be successful working in the quantum industry? Why or why not?
- What support have you received in pursuing work in the quantum industry (or industry more broadly)?
- If you were to get a job in the quantum industry in the future, do you expect that you would feel like you belong there? Why or why not?
- Would any of your answers earlier have changed if I asked you about other kinds of industry jobs outside of the quantum industry?

### Demographic Info

- Do you mind if I ask you about your gender and race and/or ethnicity? This information will be confidential to the research team.
- If yes: What race and/or ethnicity do you identify with? What is your gender? What pronouns would you like us to use when referring to your responses in a research paper or presentation?
- If no: No problem, that's fine with me.
- Are there other aspects of your identity that you feel are important that you want to share with us?

## II. SECOND AND THIRD INTERVIEW PROTOCOL

The following are the relevant parts of the interview protocol used for semi-structured interviews at the end of the first and second semesters of Q-Forge. If students did not participate in a first interview, demographic questions were also asked here.

### Background

- Have your plans for a job/career after graduation changed since the previous interview?

### Quantum Industry Specific Questions

- Tell me a little bit about what you now understand the quantum industry to be after taking this course. Do you feel like you're more familiar with what companies exist in the quantum industry after taking this course? How did you learn about these companies?
- Do you feel like you have more knowledge now of what types of jobs exist in the quantum industry than you did at the beginning of the semester? Describe some of those jobs. Of those, which would you consider/be interested in? Of those, which are you not interested in?
- Do you have more knowledge of what skills are required to work in the quantum industry? How did your knowledge of these skills change?
- If you pursued a job in the quantum industry, what do you imagine the work would be like? What parts do you expect you'd find interesting? What parts would you expect not to like?
- Are you currently interested in pursuing a job in the quantum industry? Why or why not? What parts of the course influenced this interest? How does this compare with your interest in other options (e.g., other areas of industry, academia, etc.)? How has this changed since the beginning of the semester?
- How confident are you currently in your ability to get a job in the quantum industry? Explain. What do you see as the biggest challenge to getting a job in the quantum industry? How has this changed since the beginning of the semester?
- Do you think you currently have the skills you need to be successful working in the quantum industry? Why or why not?
- What support have you received this semester in pursuing work in the quantum industry (or industry more broadly)? How has this changed since the beginning of the semester? What support do you feel like Q-Forge gave you? ‘
- Have you ever felt uncomfortable or excluded from the quantum industry or spaces or activities that would help you prepare for it this semester? In what ways? What would you need to feel like you belong in the quantum industry? Do you think you are a good fit for the quantum industry? How has this changed since the beginning of the semester?

## III. REFLECTION QUESTION PROMPTS

The following are the reflection questions related to student perceptions of the quantum industry that were asked of students throughout the course of the year. The prompts followed by an asterisk cycled through in the second semester every three weeks (3-4 times total) after the students settled into their routine of working on the industry project.

### First Semester

- Was there anything surprising you learned during the discussion about intellectual property and non-disclosure agreements? Briefly describe what it was, why you found it surprising, and how it compares with the way ideas were discussed in your prior research and/or industry experiences, if you have any.
- After doing the essential skills modules [project management modules] this week, how comfortable do you feel using industry-standard terminology to communicate what are the necessary inputs and potential outputs of your project?
- At the moment, how confident are you about your ability to contribute to the [industry] project and why?

- What did you learn from the field trip [to industry sponsor] both with respect to the quantum industry and with respect to your project?
- After starting to work on the project, has your interest in pursuing a job in the quantum industry increased, decreased, or remained the same? Please explain.
- How have your interactions with the industry partners been? What has gone well? What could be done better?
- Describe one thing you did this week that you think is authentic to a real industry experience.
- Describe one thing you did this week related to Q-Forge that you do not think is part of an authentic industry experience.
- To what extent do you feel that the support you've received from the course instructors and [the industry partner] has been adequate to ensure that you make progress on the project? Please explain.
- How are you feeling about your team's ability to make progress on the project given the updated expectations and project goals?
- You have now visited or had visitors from four local quantum companies. What have you gotten out of your interactions with various quantum industry companies aside from [the industry partner]?
- How has working on this industry project impacted your interest in pursuing a career in industry?
- After participating in this industry project, how confident do you feel in your ability to successfully work in industry? Please explain.

## Second Semester

- How did you feel about your team's communication with the industry sponsor this week?\*
- Did you do anything in the past week that helped prepare you for a job in quantum industry? If so, what was it? If not, was there anything else you did for Q-Forge that you found valuable?\*
- Did you have any experiences in the course this week that changed your level of interest in entering the quantum industry? Why or why not?\*
- What skills do you feel like you didn't gain from this course that are important to being successful in quantum industry?
- Are you planning to enter the quantum industry after graduating? Why or why not?

## IV. PHOTOVOICE PROMPTS

The following are the photovoice prompts related to students' perceptions of the quantum industry that were used throughout the Q-Forge course. The prompts followed by an asterisk were cycled through every three weeks (3-4 times total) in the second semester after the students settled into working on the industry project:

### First Semester

- Take a photo that represents the environment/culture of a company in the quantum industry.
- Take a photo representing how you feel about the project right now.
- Take a photo representing what you find most interesting at the moment about pursuing a career in quantum industry.
- Take a photo of something with respect to the [industry] project that you are proud of.

### Second Semester

- Take a photo representing your level of interest at the moment about pursuing a career in quantum industry.\*

## V. PHOTOVOICE FOCUS GROUP PROTOCOL

The following questions were asked of the students with respect to each category of photos during each of the focus groups:

- What themes do you notice in these photos?
- How do these themes represent your collective experience with quantum industry/the course as a whole?
- Do any of the comments other people made about your photos resonate with you? Were there any comments that surprised you?
- After hearing from the photographers, are there any changes you want to make to the list of themes you noticed in the photos?
